# Supplementary material for: Designing Equitable Transit Networks
Source: arXiv:2212.12007 source file (2023-08-07)
Supplement: Supplementary file 1 [file appendix.tex]

\section{Supplementary Results}
\input{plots/BarPlots.tex}

\subsection{Demand Distribution}

In Figure~\ref{fig:Demand}, we present the distribution of the travel demand among the priority groups in both Chattanooga, Hamilton county, and Franklin, Williamson county. Recall that in our formulation, ``priority group 1'' denotes the highest priority. In both cities, we see the most demand comes from group 3. The key difference between the demand profiles is that for Franklin, the demand is skewed more toward higher priority groups, i.e., a larger portion of the demand originates from the high-priority groups. 

The supplementary material consists of several figures. We present all figures after the text. Instead of explaining each figure separately, we point out the general trends and inferences based on the experiments. Further, for all experimental results (including the main text), we set $\gamma = 0.01$ for formulations labeled as ``Rawlsian'' in order to make the objective of our optimization problem monotonic increasing (refer to section~\ref{section: social welfare functions} in the main text).

\subsection{Exploring Linear Combinations of Utilitarian and Rawlsian Objectives (Chattanooga)}
In the main body of the paper, we evaluated the effects of the Rawlsian formulation and the utilitarian formulation on balancing ridership and coverage in the context of public transit. Here, we begin by evaluating multiple linear combinations of the two social welfare functions, weighed by the parameter $\gamma$. We seek to evaluate: \textit{how does differing values of $\gamma$ affect the average utility with different considerations of priorities?}

\begin{figure*}[ht]
\centering
\begin{subfigure}[b]{.33\textwidth}
\resizebox{1\columnwidth}{!}{
\input{plots/line_plot/chattanooga/center/LinearCombo/gamma0.1/EP.tex}}
\caption{Equal Priorities}
\end{subfigure}\hfill
\begin{subfigure}[b]{.33\textwidth}
\resizebox{1\columnwidth}{!}{
\input{plots/line_plot/chattanooga/center/LinearCombo/gamma0.1/P.tex}}
\caption{Unequal Priorities}
\end{subfigure}\hfill
\begin{subfigure}[b]{.33\textwidth}
\resizebox{1\columnwidth}{!}{
\input{plots/line_plot/chattanooga/center/LinearCombo/gamma0.1/difference.tex}}
\caption{Utility Gain} 
\end{subfigure}
\caption{Average Utility and Gain based on the Linear Combination Formulation, $\gamma = 0.1$: Chattanooga, Hamilton County, TN}
\label{fig:ChattLC1}
\end{figure*}

% \begin{figure*}[ht]
% \centering
% \begin{subfigure}[b]{.33\textwidth}
% \resizebox{1\columnwidth}{!}{
% \input{plots/line_plot/chattanooga/center/LinearCombo/gamma0.3/EP.tex}}
% \caption{Equal Priorities}
% \end{subfigure}\hfill
% \begin{subfigure}[b]{.33\textwidth}
% \resizebox{1\columnwidth}{!}{
% \input{plots/line_plot/chattanooga/center/LinearCombo/gamma0.3/P.tex}}
% \caption{Unequal Priorities}
% \end{subfigure}\hfill
% \begin{subfigure}[b]{.33\textwidth}
% \resizebox{1\columnwidth}{!}{
% \input{plots/line_plot/chattanooga/center/LinearCombo/gamma0.3/difference.tex}}
% \caption{Utility Gain} 
% \end{subfigure}
% \caption{Average Utility and Gain based on the Linear Combination Formulation, $gamma = $0.3: Chattanooga, Hamilton County, TN}
% \label{fig:ChattLC3}
% \end{figure*}

\begin{figure*}[ht]
\centering
\begin{subfigure}[b]{.33\textwidth}
\resizebox{1\columnwidth}{!}{
\input{plots/line_plot/chattanooga/center/LinearCombo/gamma0.5/EP.tex}}
\caption{Equal Priorities}
\end{subfigure}\hfill
\begin{subfigure}[b]{.33\textwidth}
\resizebox{1\columnwidth}{!}{
\input{plots/line_plot/chattanooga/center/LinearCombo/gamma0.5/P.tex}}
\caption{Unequal Priorities}
\end{subfigure}\hfill
\begin{subfigure}[b]{.33\textwidth}
\resizebox{1\columnwidth}{!}{
\input{plots/line_plot/chattanooga/center/LinearCombo/gamma0.5/difference.tex}}
\caption{Utility Gain} 
\end{subfigure}
\caption{Average Utility and Gain based on the Linear Combination Formulation, $\gamma = 0.5$: Chattanooga, Hamilton County, TN}
\label{fig:ChattLC5}
\end{figure*}

\begin{figure*}[ht]
\centering
\begin{subfigure}[b]{.33\textwidth}
\resizebox{1\columnwidth}{!}{
\input{plots/line_plot/chattanooga/center/LinearCombo/gamma0.7/EP.tex}}
\caption{Equal Priorities}
\end{subfigure}\hfill
\begin{subfigure}[b]{.33\textwidth}
\resizebox{1\columnwidth}{!}{
\input{plots/line_plot/chattanooga/center/LinearCombo/gamma0.7/P.tex}}
\caption{Unequal Priorities}
\end{subfigure}\hfill
\begin{subfigure}[b]{.33\textwidth}
\resizebox{1\columnwidth}{!}{
\input{plots/line_plot/chattanooga/center/LinearCombo/gamma0.7/difference.tex}}
\caption{Utility Gain} 
\end{subfigure}
\caption{Average Utility and Gain based on the Linear Combination Formulation, $\gamma = 0.7$: Chattanooga, Hamilton County, TN}
\label{fig:ChattLC7}
\end{figure*}

\begin{figure*}[htbp]
\centering
\begin{subfigure}[b]{.33\textwidth}
\resizebox{1\columnwidth}{!}{
\input{plots/line_plot/franklin/center/Utilitarian/EP.tex}}
\caption{Equal Priorities}
\end{subfigure}\hfill
\begin{subfigure}[b]{.33\textwidth}
\resizebox{1\columnwidth}{!}{
\input{plots/line_plot/franklin/center/Utilitarian/P.tex}}
\caption{Unequal Priorities}
\end{subfigure}\hfill
\begin{subfigure}[b]{.33\textwidth}
\resizebox{1\columnwidth}{!}{
\input{plots/line_plot/franklin/center/Utilitarian/difference.tex}}
\caption{Utility Gain} 
\end{subfigure}
\caption{Average Utility and Gain based on the Utilitarian Formulation: Franklin, Williamson County, TN}
\label{fig:UtilitarianFrank}
\end{figure*}

\begin{figure*}[htbp]
\centering
\begin{subfigure}[b]{.33\textwidth}
\resizebox{1\columnwidth}{!}{
\input{plots/line_plot/franklin/center/MaxMin/EP.tex}}
\caption{Equal Priorities}
\end{subfigure}\hfill
\begin{subfigure}[b]{.33\textwidth}
\resizebox{1\columnwidth}{!}{
\input{plots/line_plot/franklin/center/MaxMin/P.tex}}
\caption{Unequal Priorities}
\end{subfigure}\hfill
\begin{subfigure}[b]{.33\textwidth}
\resizebox{1\columnwidth}{!}{
\input{plots/line_plot/franklin/center/MaxMin/difference.tex}}
\caption{Utility Gain} 
\end{subfigure}
\caption{Average Utility and Gain based on the Rawlsian Formulation: Franklin, Williamson County, TN}
\label{fig:MaxMinFrank}
\end{figure*}

% \begin{figure*}[ht]
% \centering
% \begin{subfigure}[b]{.33\textwidth}
% \resizebox{1\columnwidth}{!}{
% \input{plots/line_plot/chattanooga/center/Utilitarian/EP.tex}}
% \caption{Equal Priorities}
% \end{subfigure}\hfill
% \begin{subfigure}[b]{.33\textwidth}
% \resizebox{1\columnwidth}{!}{
% \input{plots/line_plot/chattanooga/center/Utilitarian/P.tex}}
% \caption{Unequal Priorities}
% \end{subfigure}\hfill
% \begin{subfigure}[b]{.33\textwidth}
% \resizebox{1\columnwidth}{!}{
% \input{plots/line_plot/chattanooga/center/Utilitarian/difference.tex}}
% \caption{Utility Gain} 
% \end{subfigure}
% \caption{Average Utility and Gain based on the Utilitarian Formulation: Chattanooga, Hamilton County, TN}
% \label{fig:Utilitarian}
% \end{figure*}

% \begin{figure*}[ht]
% \centering
% \begin{subfigure}[b]{.33\textwidth}
% \resizebox{1\columnwidth}{!}{
% \input{plots/line_plot/chattanooga/center/MaxMin/EP.tex}}
% \caption{Equal Priorities}
% \end{subfigure}\hfill
% \begin{subfigure}[b]{.33\textwidth}
% \resizebox{1\columnwidth}{!}{
% \input{plots/line_plot/chattanooga/center/MaxMin/P.tex}}
% \caption{Unequal Priorities}
% \end{subfigure}\hfill
% \begin{subfigure}[b]{.33\textwidth}
% \resizebox{1\columnwidth}{!}{
% \input{plots/line_plot/chattanooga/center/MaxMin/difference.tex}}
% \caption{Utility Gain} 
% \end{subfigure}
% \caption{Average Utility and Gain based on the Rawlsian Formulation: Chattanooga, Hamilton County, TN}
% \label{fig:MaxMin}
% \end{figure*}
%lc 0.1
\begin{figure*}[htbp]
\centering
\begin{subfigure}[b]{.33\textwidth}
\resizebox{1\columnwidth}{!}{
\input{plots/line_plot/franklin/center/LinearCombo/gamma0.1/EP.tex}}
\caption{Equal Priorities}
\end{subfigure}\hfill
\begin{subfigure}[b]{.33\textwidth}
\resizebox{1\columnwidth}{!}{
\input{plots/line_plot/franklin/center/LinearCombo/gamma0.1/P.tex}}
\caption{Unequal Priorities}
\end{subfigure}\hfill
\begin{subfigure}[b]{.33\textwidth}
\resizebox{1\columnwidth}{!}{
\input{plots/line_plot/franklin/center/LinearCombo/gamma0.1/difference.tex}}
\caption{Utility Gain} 
\end{subfigure}
\caption{Average Utility and Gain based on the Linear Combination Formulation, $\gamma = 0.1$: Franklin, Williamson County, TN}
\label{fig:FrankLC1}
\end{figure*}

%lc 0.5
\begin{figure*}[htbp]
\centering
\begin{subfigure}[b]{.33\textwidth}
\resizebox{1\columnwidth}{!}{
\input{plots/line_plot/franklin/center/LinearCombo/gamma0.5/EP.tex}}
\caption{Equal Priorities}
\end{subfigure}\hfill
\begin{subfigure}[b]{.33\textwidth}
\resizebox{1\columnwidth}{!}{
\input{plots/line_plot/franklin/center/LinearCombo/gamma0.5/P.tex}}
\caption{Unequal Priorities}
\end{subfigure}\hfill
\begin{subfigure}[b]{.33\textwidth}
\resizebox{1\columnwidth}{!}{
\input{plots/line_plot/franklin/center/LinearCombo/gamma0.5/difference.tex}}
\caption{Utility Gain} 
\end{subfigure}
\caption{Average Utility and Gain based on the Linear Combination Formulation, $\gamma = 0.5$: Franklin, Williamson County, TN}
\label{fig:FrankLC5}
\end{figure*}

%lc 0.7
\begin{figure*}[ht]
\centering
\begin{subfigure}[b]{.33\textwidth}
\resizebox{1\columnwidth}{!}{
\input{plots/line_plot/franklin/center/LinearCombo/gamma0.7/EP.tex}}
\caption{Equal Priorities}
\end{subfigure}\hfill
\begin{subfigure}[b]{.33\textwidth}
\resizebox{1\columnwidth}{!}{
\input{plots/line_plot/franklin/center/LinearCombo/gamma0.7/P.tex}}
\caption{Unequal Priorities}
\end{subfigure}\hfill
\begin{subfigure}[b]{.33\textwidth}
\resizebox{1\columnwidth}{!}{
\input{plots/line_plot/franklin/center/LinearCombo/gamma0.7/difference.tex}}
\caption{Utility Gain} 
\end{subfigure}
\caption{Average Utility and Gain based on the Linear Combination Formulation, $\gamma = 0.7$: Franklin, Williamson County, TN}
\label{fig:FrankLC7}
\end{figure*}
\begin{figure*}[ht]
\centering
\begin{subfigure}[b]{.33\textwidth}
\resizebox{1\columnwidth}{!}{
\input{plots/line_plot/franklin/center/difference/MaxMinEP_UEP.tex}}
\caption{Rawlsian Equal Priorities}
\label{r_ep_f}
\end{subfigure}\hfill
\begin{subfigure}[b]{.33\textwidth}
\resizebox{1\columnwidth}{!}{
\input{plots/line_plot/franklin/center/difference/MaxMinP_UEP.tex}}
\caption{Rawlsian Unequal Priorities}
\label{r_p_f}
\end{subfigure}\hfill
\begin{subfigure}[b]{.33\textwidth}
\resizebox{1\columnwidth}{!}{
\input{plots/line_plot/franklin/center/Utilitarian/service_EP.tex}}
\caption{Percentage of People Served} 
\label{u_ep_f}
\end{subfigure}
\caption{(\subref{r_ep_f}) (\subref{r_p_f}) The gain in average utility compared to a utilitarian baseline, and (\subref{u_ep_f}) Percentage of people served by the utilitarian baseline in Franklin, Williamson County, TN.}
\label{fig:ServeBase_Frank}
\end{figure*}

% \noindent \textbf{Differing Combinations:}
As in the main text, we first present all results for the city of Chattanooga, Hamilton county. We set $\gamma = \{0.1, 0.5, 0.7\}$, and present the results in Figures~\ref{fig:ChattLC1}, \ref{fig:ChattLC5} and \ref{fig:ChattLC7}, respectively. Recall that $0 \leq \gamma \leq 1$, where a value of $\gamma = 0.5$ signifies an equal combination of the two social welfare functions, and a value of $\gamma < 0.5$ weighs in favor of the Rawlsian formulation. Here, we observe the average utility for all origin-destination pairs with and without the notion of priority by varying $\gamma$ to higher values.

% We observe that the relative gain for each combination by accounting for priorities as done for Utilitarian and Rawlsian formulations. 
We observe similar results as for the individual formulations, where the notion of priorities does not make any difference at higher budgets, as all origin-destination pairs can be served through a path of length close (if not exactly equal) to their shortest paths. We are interested in the behavior at the lower budgets as we vary $\gamma$. As $\gamma$ increases, we observe an increase in cumulative average utility at lower budgets when priorities are not explicitly modeled. Figure \ref{fig:ChattLC7} (b) demonstrates using heterogeneous priority scores with a higher $\gamma$, all priority scores will have a higher average utility at lower budgets, compared to models with smaller values of $\gamma$, such as Figures \ref{fig:ChattLC1} (b) and \ref{fig:ChattLC5} (b). This can be explained as the gap between the highest priority group and lowest priority group being tightened at low budgets (when priorities are considered). This is due to the combination weighing in favor of the utilitarian formulation, which favors a maximization of ridership. 
% \textcolor{red}{Ayan: which figure is the steep decrease referring to? What is it relative to? Just Utilitarian?}
% \textcolor{red}{Sophie: Figure 6b, when gamma 0.5, steep decrease for lower priority groups at lower budgets}

% where the cumulative gain in utility offsets any potential gain from considering the notion of priority. 

\noindent \textbf{Key Takeaways:}
We observe that as the value of $\gamma$ increases, the resulting network design is dominated by the utilitarian objective of maximizing ridership. At lower values of $\gamma$, while the group of origin-destination pairs who need transit the most can have a significant gain in utility, this gain comes at the cost of a reduction of utility of the other groups. 

\subsection{Evaluation on Franklin, Williamson County}
In addition to presenting the linear combination results for Franklin, Williamson County, we include results for the Utilitarian and Rawlsian formulations.

\noindent \textbf{Utilitarian formulation:}
We observe similar results when comparing the utilitarian formulation for Chattanooga and Franklin. Figure~\ref{fig:UtilitarianFrank} shows the average utility across the origin-destination pairs with and without the notion of priority for the utilitarian objective. Figure~\ref{fig:UtilitarianFrank} (c) demonstrates the relative gain in average utility for each priority group by choosing the model where priorities are explicitly modeled. We observe that when priorities are considered, the utilitarian formulation results in relative gains for the group with the highest priority at lower budgets. At higher budgets, however, there is no significant relative gain in average utility. This observation is true to our finding in Figure~\ref{fig:Utilitarian}.

\noindent \textbf{Rawlsian formulation:}
 We present results for the Rawlsian formulation for the city of Franklin in Figure~\ref{fig:MaxMinFrank}. We observe that without accounting for priorities, the resulting network results in the highest utility for priority group 4 (recall that group 1 denotes the highest priority). We hypothesize that this gain largely comes from the fact that there is a very small fraction of the population in this group, and although the group has people with high rates of car ownership and household income, they reside in areas that are difficult to serve. However, accounting for priorities ensures that the group that depends on public transit more critically is served with the highest average utility.

\subsection{Exploring Linear Combinations of Utilitarian and Rawlsian Objectives (Franklin)}

We solve the equitable network design problem with $\gamma=\{0.1,0.5,0.7\}$ and present results in Figures \ref{fig:FrankLC1}, \ref{fig:FrankLC5} and \ref{fig:FrankLC7}. Observe that when priorities are not accounted, the origin-destination pairs from priority group 4 have the lowest average utility in the utilitarian formulation (see Figure~\ref{fig:UtilitarianFrank} (a)). As we pointed out earlier, this observation is driven by a very low fraction of people belonging to group 4, who are difficult to serve when maximizing ridership (i.e., utilitarian objective). However, even a small component of the Rawlsian formulation ($\gamma=0.1$ (see Figure~\ref{fig:FrankLC1} (a)) results in a massive gain in utility for group 4. While this points out the benefits of using a Rawlsian formulation, it also reveals that not accounting for priorities might result in high average utility for a group that does not depend on public transit critically. When priorities are considered explicitly (see Figure~\ref{fig:FrankLC1} (b)), origin-destination pairs from group 1 (the group which needs transit the most based on our priority function) achieve the highest utility. As $\gamma$ is increased, we observe this trend more clearly, i.e., group 4 achieves the highest utility when priorities are not considered (Figures~\ref{fig:FrankLC5} (a) and Figures~\ref{fig:FrankLC7} (a)). However, by explicitly accounting for priorities, the gains shift to group 1, with a massive drop in utility for group 4. 

\noindent \textbf{Key Takeaways:} Our experiments on the city of Franklin reveal several key lessons. First, formulations based solely on a utilitarian formulation can sacrifice utility for a group that is hard to serve. This is further shown in Figure~\ref{fig:ServeBase_Frank} (c), which shows that in a purely utilitarian formulation, the percentage of people served for group 4 is very low. However, using a Rawlsian formulation can result in restoring high average utility for such a group (see Figure~\ref{fig:ServeBase_Frank} (a), which shows a very high gain for group 4 with respect to the ``business-as-usual'' model). Crucially, the group in consideration can be composed of a very small number of residents who might not ``need'' public transit, i.e., they have high incomes and high rates of car ownership. Therefore, accounting for priorities explicitly is critical in ensuring that the section of the population that needs transit the most is served.
% \section{Notation}
% \input{plots/BarPlots.tex}
